# Supplementary material for: Origin of Biquadratic Exchange Interactions in a Mott Insulator as a Driving Force of Spin Nematic Order
Source: arXiv:1805.07911 source file (2018-05-21)
Supplement: Supplementary file 1 [file supplementalmaterial.pdf]

# Supplemental Material for "Origin of Biquadratic Exchange Interactions in a Mott Insulator as a Driving Force of Spin Nematic Order"

Katsuhiro Tanaka, Yuto Yokoyama, and Chisa Hotta

*Department of Basic Science, University of Tokyo, 3-8-1 Komaba, Meguro, Tokyo 153-8902, Japan*

## 1 Interaction coefficients for Case (i)

While only the sums of the parameters are shown in the main text, we compare each interaction parameter appeared in Case (i) below (see Fig. S1).

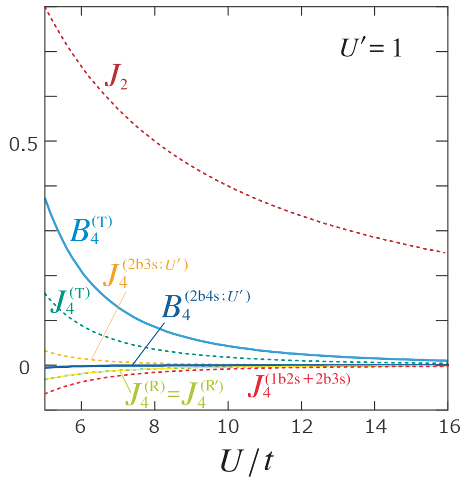


Fig. S1: Evaluation of model parameters in Case (i) as a function of $U/t$. We set $U' = 1$ and $t = t' = t'' = 1$.

## 2 Interaction coefficients from 4th order perturbation for Case (ii)

Here we note the interaction coefficients of the bilinear (Heisenberg) interaction $\hat{S}_i \cdot \hat{S}_j$, and the biquadratic interaction $\left(\hat{S}_i \cdot \hat{S}_j\right)^2$, for *2-site-2 orbital system* (Case (ii)). We include $J_p \neq 0$ in the following equations, although only part of the terms at $J_p = 0$ is given in the main text.

### Bilinear (Heisenberg) interactions

Each element of $J_4^{(\mathrm{process})}$ is expressed as follows;

$$J_4^{(T)} = t^2 t'^2 \left[ -\frac{12}{(U+J_H)^2(U-2J_H-J_p)} - \frac{4}{(U-2J_H-J_p)^2(U+J_H)} \right], \tag{S1}$$

$$J_4^{(2b4s)} = \frac{t^4 + t'^4}{2} \left[ -\frac{8}{(U+J_H)^3} + \frac{6}{(U+J_H)^2(U-J_H)} + \frac{2}{(U+J_H)(U-J_H)^2} \right], \tag{S2}$$

$$J_4^{(1b2s)} = \frac{t^4 + t'^4}{2} \left[ -\frac{8}{(U+J_H)^3} - \frac{6}{(U+J_H)^2(U-J_H)} - \frac{2}{(U+J_H)(U-J_H)^2} \right], \tag{S3}$$

$$J_4^{(2b3s)} = t^2 t'^2 \left[ -\frac{16}{(U+J_H)^3} - \frac{12}{(U+J_H)^2(U-2J_H-J_p)} - \frac{4}{(U+J_H)(U-2J_H-J_p)^2} \right]. \tag{S4}$$

**Biquadratic interactions**

Each element of $B_4^{(\mathrm{process})}$ is expressed as follows ($B_4^{(\mathrm{T})}$ and $B_4^{(\mathrm{2b4s})}$ are appeared also in the main text);

$$B_4^{(\mathrm{T})} = t^2t'^2\left[-\frac{12}{(U+J_H)^2(U-4J_H-J_p)} - \frac{4}{(U-4J_H-J_p)^2(U+J_H)} + \frac{4}{(U+J_H)^2(U-J_H)} - \frac{12}{(U+J_H)^2(U-2J_H-J_p)} - \frac{4}{(U-2J_H-J_p)^2(U+J_H)}\right], \tag{S5}$$

$$B_4^{(\mathrm{2b4s})} = \frac{t^4+t'^4}{2}\left[\frac{4}{(U+J_H)^3} + \frac{6}{(U+J_H)^2(U-5J_H+2J_p)} + \frac{6}{(U+J_H)^2(U-5J_H-2J_p)} + \frac{2}{(U+J_H)(U-5J_H+2J_p)^2} + \frac{2}{(U+J_H)(U-5J_H-2J_p)^2} + \frac{2}{(U+J_H)^2(U-J_H)} + \frac{2}{(U+J_H)(U-J_H)^2} + \frac{3}{(U+J_H)^2(U-3J_H)} + \frac{1}{(U+J_H)(U-3J_H)^2}\right], \tag{S6}$$

$$B_4^{(\mathrm{1b2s})} = \frac{t^4+t'^4}{2}\left[\frac{4}{(U+J_H)^3} - \frac{6}{(U+J_H)^2(U-J_H)} - \frac{2}{(U+J_H)(U-J_H)^2} + \frac{3}{(U+J_H)^2(U-3J_H)} + \frac{1}{(U+J_H)(U-3J_H)^2}\right], \tag{S7}$$

$$B_4^{(\mathrm{2b3s})} = t^2t'^2\left[\frac{8}{(U+J_H)^3} - \frac{6}{(U+J_H)^2(U-3J_H)} - \frac{2}{(U+J_H)(U-3J_H)^2} - \frac{12}{(U+J_H)^2(U-2J_H-J_p)} - \frac{4}{(U+J_H)(U-2J_H-J_p)^2} + \frac{12}{(U+J_H)^2(U-4J_H-J_p)} + \frac{4}{(U+J_H)(U-4J_H-J_p)^2}\right]. \tag{S8}$$

Figure S2 shows the comparison of the interaction parameters in Eqs. (S1)–(S8) at $J_p = 0$.

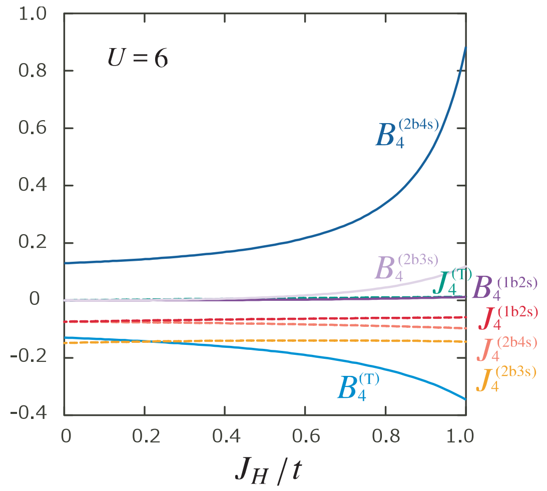


Fig. S2: Evaluation of model parameters in Eqs. (S1)–(S8) as a function of $J_H/t$ at $U = 6$ and $J_p = 0$. We set $t = t' = 1$.
